# Supplementary material for: Mirror Surface Nanostructuring via Laser Direct Writing -- Characterization and Physical Origins
Source: arXiv:2211.05096 source file (2022-11-09)
Supplement: Supplementary file 1 [file suppmat.pdf]

# 1 Mirror structure

A sketch of the nanostructurable mirror is shown in **Figure A1**.
In order to evaluate mirrors with a dielectric stack that has fewer than 20 $Ta_2O_5$ and $SiO_2$ pairs, we use superglue to attach a piece of aluminium to the mirror surface. Then we forcefully detach it with pliers which removes a certain number of layers, but appears to leave the underlying structure intact. After a few attempts we got an area that had an $11 \pm 1$ pair dielectric stack and was large enough to perform the calibration on.

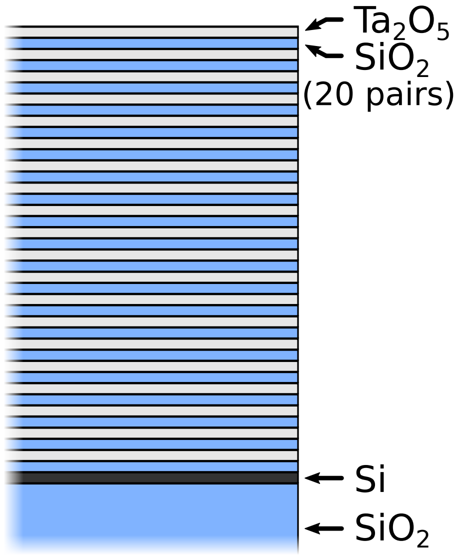


Figure A1: Nanostructurable dielectric mirrors consisting of a fused silica substrate, an amorphous silicon layer, and 20 pairs of $Ta_2O_5$ and $SiO_2$. Not to scale.

# 2 The nanostructuring setup

The permanent nanostructuring of mirrors with the additional absorptive layer is performed in a standalone setup with integrated surface evaluation. The benefit of this is that such a specialized setup may be then shared between multiple (photon BEC) experiments. There are several things to be considered in the design of such a setup.

Firstly, the side from which the writing laser beam impinges onto the absorptive layer. Back-side writing has the benefit of a somewhat higher absorption, but reduced viable writing area as the focused beam is at risk of being partially cut off while traversing the substrate. Front-side writing, on the other hand, constrains the writing laser wavelength to lie in the transmissive region of the mirror. It is also more sensitive to dust that may find itself in the nanostructured area. The main benefit is the fact that the surface evaluation and the writing optics may be combined, increasing the accuracy of alignment and focusing, as well as reducing the setup size. Overall, both methods work and achieve similar results.

The second consideration concerns the writing procedure as such. Using focused Gaussian beams and writing point by point is the easiest way to construct complex structures, and the one we employ. In this case, the limiting factor for the writing speed is usually the translational stages. It would be possible to use higher optical powers combined with wavefront shaping, galvo or polygon mirror scanners to speed up writing, however for small-scale usage this appears to be unnecessary, as 100 $\mu m^2$ structures can be written in minutes. The writing procedure depends on three parameters: the focus, the beam power, and the pulse duration. The focus determines the beam size at the thin silicon layer, and combined with beam power determines the irradiance. Both the written point height and full width at half maximum (FWHM) depend on these three parameters in a non-trivial way. A reasonable approach is to keep the beam power constant, and only vary the focus and pulse duration.

The final consideration is the optical characterization of the surface height profile: white light interferometry provides a sufficiently high resolution and can be easily implemented using a Mirau interferometric objective, which is what we use.

The full schematic of the nanostructuring setup is shown in **Figure A2**a.
The setup is assembled within an aluminium frame (dimensions 22 x 31 x 34 cm) enclosed in acrylic sheets, standing on Sorbothane pads (see **Figure A2**c). The enclosure helps reduce dust build-up, and provides shielding against the violet writing laser light. The pulse timing and stage synchronization is implemented on a single board computer: the Red Pitaya, which has an embedded FPGA. The interferometric surface profiling provides a resolution better than 0.1 nm that is roughly the diameter of a single atom, which may be further improved by averaging multiple scans.

The target test structure used for complex structure evaluation is shown in **Figure A2**b. As described in the main text, it consists of sharp features of various heights.

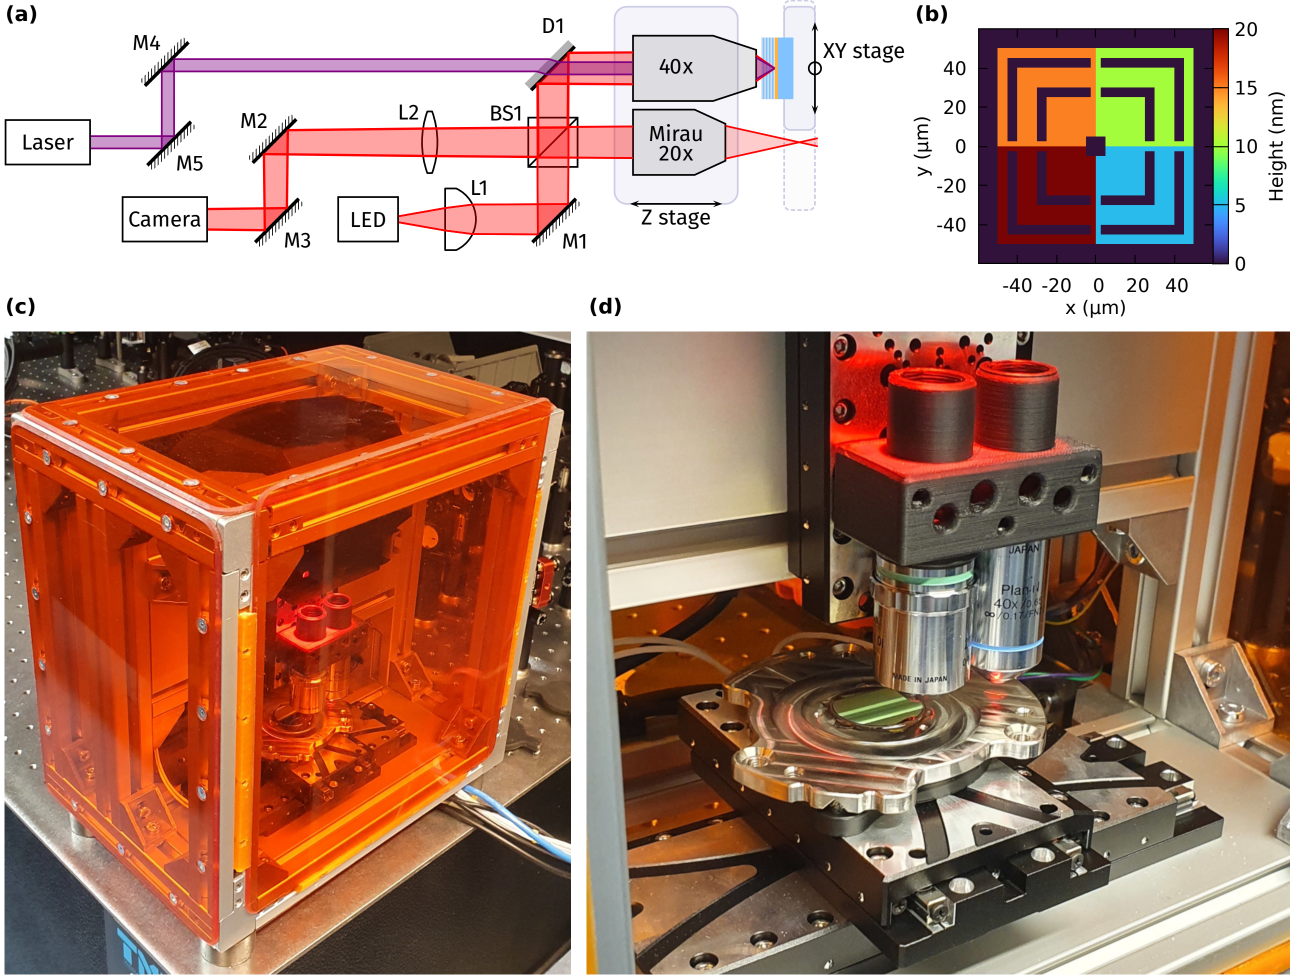


Figure A2: a) Full optical schematic of the nanostructuring setup. b) Test structure design height map. c) Picture of the enclosed setup. d) A close-up image of the translational stages, the sample mirror, and the microscope objectives.

The direct laser writing is performed by loading the target height map (as defined by an image file), converting it to a pulse duration matrix using the calibration obtained with plateau measurements, and then performing the write. The pulse duration - height mapping is obtained by fitting B-splines with an arbitrary number of knots with optimized positions to the plateau height data, which is shown in **Figure A3**.

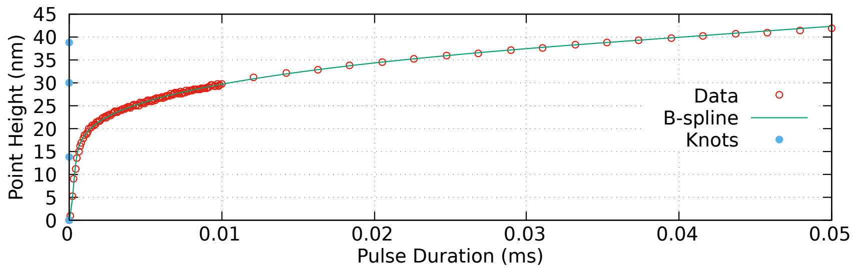


Figure A3: Calibration mapping. Pulse duration to point height mapping.

# 3 Time-resolved measurements

The full schematic of the time-resolved measurement setup is shown in **Figure A4**. In addition to the description in the main text: a filter is added to remove any transmitted 405 nm light, ensuring that only the interference pattern is imaged. One of the MZI outputs is imaged onto the camera, and the other onto a photomultiplier tube (PMT) through a pinhole. The purpose of the latter is to provide feedback for the piezo, in order to maximize interferometric sensitivity prior to measurement. The piezo is also used for determining the minimum and maximum of the signal (i.e. visibility) needed for height conversion.

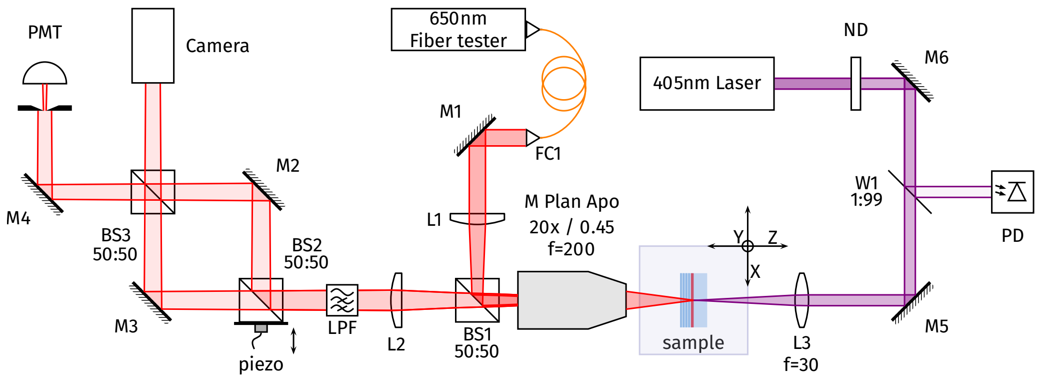


Figure A4: Full optical schematic of the time-resolved measurement setup

## 3.1 Data processing

Here we briefly describe the data processing performed on the time-resolved measurements. The camera captures a snapshot of the interference pattern in a 12 bit image. In order to convert this to height, measurements of maximum and minimum value per each pixel are performed beforehand by varying the length of one of the interferometer arms. The following equation is then used for the conversion:

$$h(i,j) = \frac{\lambda}{4\pi} \arccos\left(1 - 2\frac{I(i,j) - I_{\min}(i,j)}{I_{\max}(i,j) - I_{\min}(i,j)}\right), \tag{1}$$

where $h(i,j)$ is the height at pixel (i,j), $\lambda$ is the imaging laser wavelength, while $I(i,j)$, $I_{\min}(i,j)$ and $I_{\max}(i,j)$ are the raw pixel values. For each frame individually, the rightmost and leftmost flat regions are used as a baseline, and their average height is subtracted from the whole image which removes phase differences between frames caused by vibrations. Furthermore, for each individual pixel the average value prior to pulse start is subtracted from all the frames, which corrects the non-uniform wavefront phase. In the case of reversible pulses, averaging over corresponding frames is performed, providing the final result. The FWHM is determined by calculating the area that is above half maximum, and then determining the diameter of an circle of the same area.

## 3.2 Additional data evaluation

An alternative plot of the measurements with pulse durations of 0.3 and 8 ms is shown in **Figure A5**. Here, each pixel represents the average height of all vertical pixels per height map column. While the height value itself may be somewhat misleading, the plot helps visualize the temporal and spatial progression of the height profile.

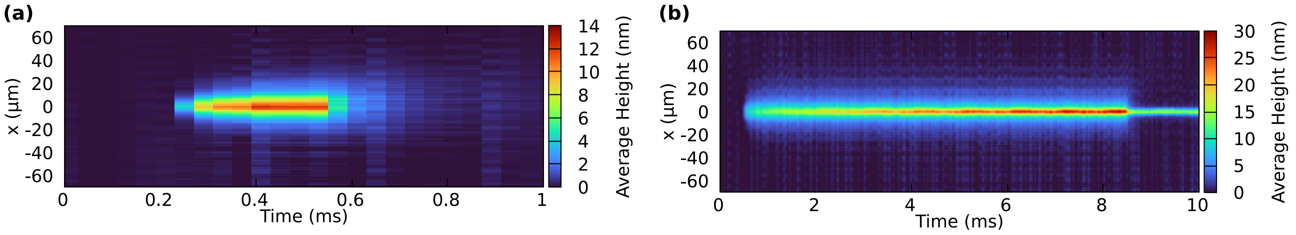


Figure A5: Time-resolved measurement results - surface plot. Results for a pulse duration of a) 0.3 and b) 8 ms, showing the height average over all measured vertical (y axis) pixels of the original height map, plotted as a function of the horizontal (x axis) position and time.

# 4 Physical origin of the nanostructuring process

Here we provide additional maps and SEM images of the nanostructured mirror cross section.

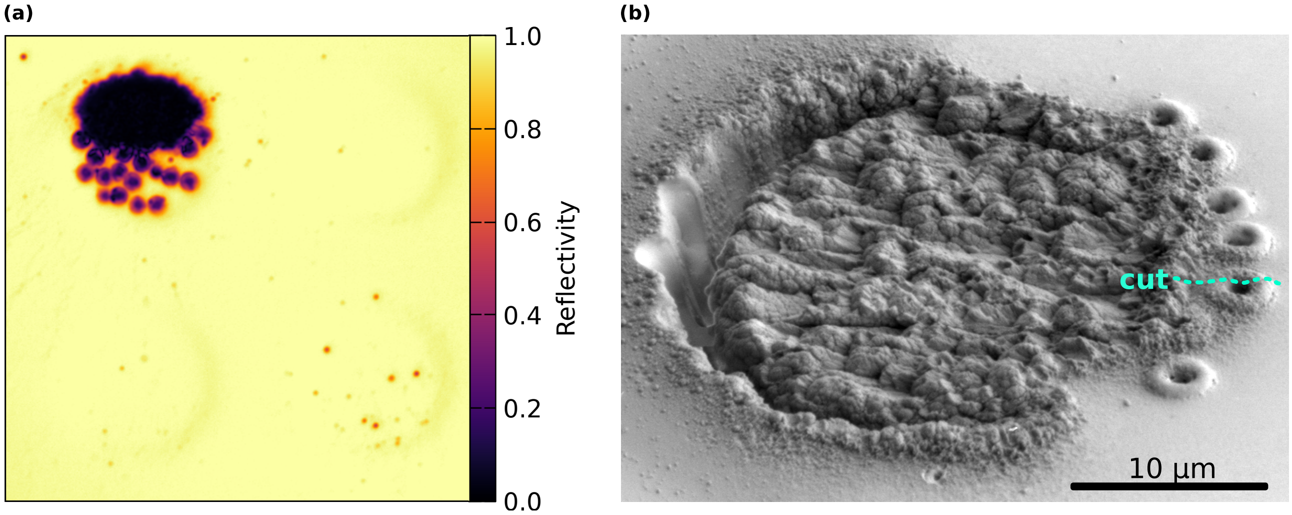


Figure A6: a) Spatially resolved reflectivity, showing the effects of mirror destruction when writing plateaus in-focus (-2 µm) with excessive pulse durations. Material ejected during the writing is seen deposited around the destroyed structure. b) A surface SEM image of a similar destroyed structure. The cyan dashed line indicates the cross section cut location of the scan shown in **Figure 6**c of the main text. Scan performed at an angle of 52 degrees. Scan courtesy of M. Goodwin.

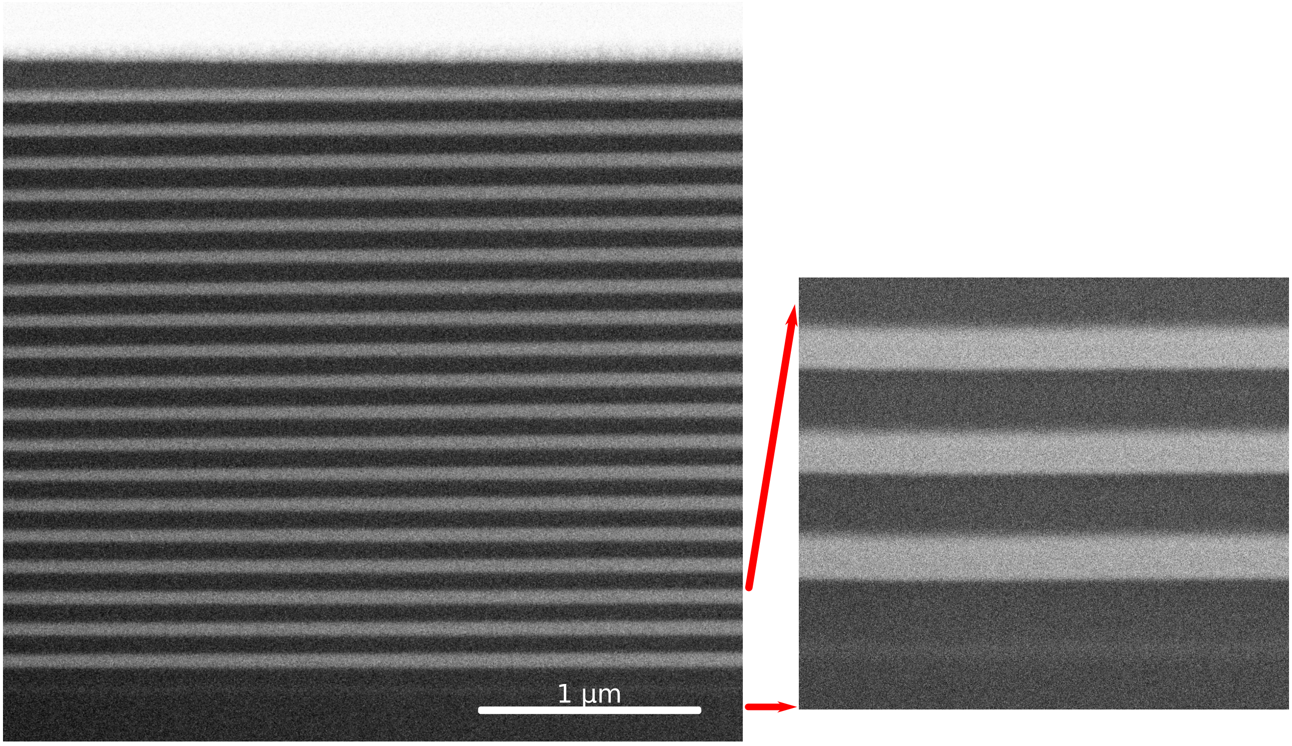


Figure A7: SEM image of the mirror cross section for a 40 nm high plateau written at z= -40 µm, with the lowermost layer area magnified in the right-hand side image (separate scan). No bubbles are resolvable in this case. The imaging angle is 52° in relation to the mirror normal. Scans courtesy of M. Goodwin.

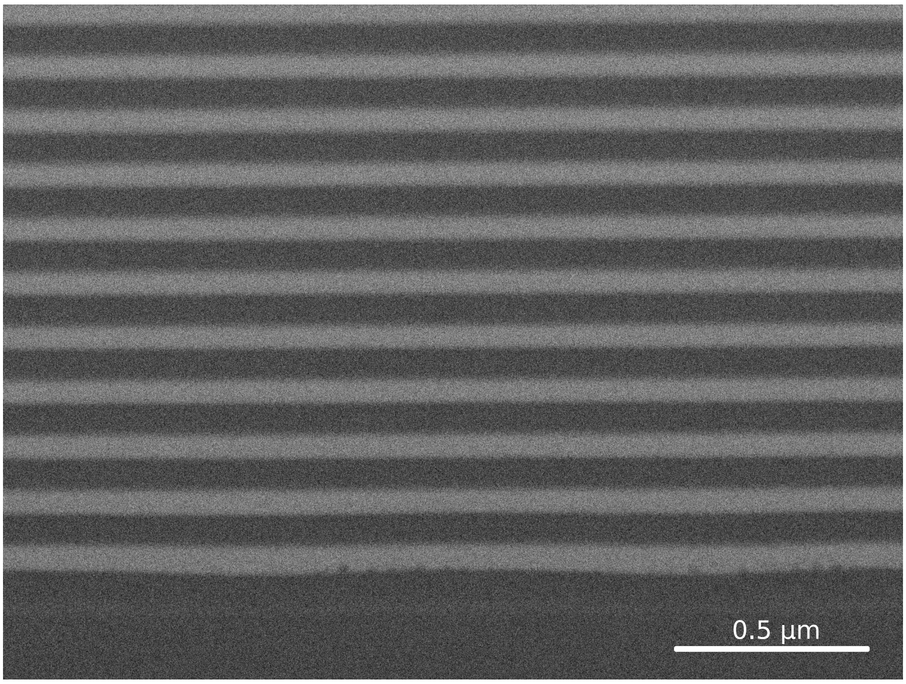


Figure A8: SEM image of the mirror cross section for an approx. 10 nm high plateau written at z= -2 µm. Some bubbles are can be observed in this case. The imaging angle is 52° in relation to the mirror normal. Scan courtesy of M. Goodwin.

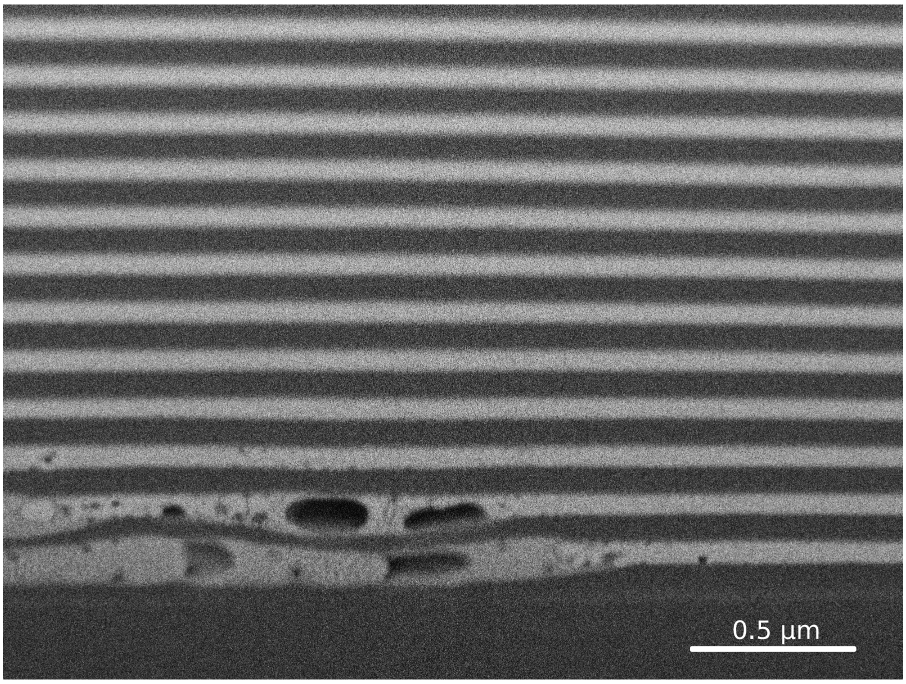


Figure A9: SEM image of the mirror cross section at the edge of a delaminated plateau written at z= -9 µm. Delamination occurs further to the left (not visible), while on the right-hand side we have a transition to the non-structured area. The imaging angle is 52° in relation to the mirror normal. Scan courtesy of M. Goodwin.
